# Supplementary material for: Dynamics of anchored oscillating nanomenisci
Source: arXiv:1706.02068 source file (2017-06-07)
Supplement: Supplementary file 1 [file SM.pdf]

# Supplemental material

# Dynamics of an anchored oscillating nanomenisci

Caroline Mortagne, [1,2] Kévin Lippera,[1,3] Philippe Tordjeman,[2] Michael Benzaquen,[3] Thierry Ondarçuhu[1]

*[1] Nanosciences group, CEMES-CNRS, 29 rue Jeanne Marvig,
31055 Toulouse Cedex 4 France*

*[2] IMFT - Université de Toulouse, CNRS-INPT-UPS, 1 allée du Professeur Camille Soula,
31400 Toulouse France*

*[3] LadHyX - Ecole Polytechnique, CNRS, Boulevard des Maréchaux,
91120 Palaiseau, France*

**SM1: Tip fabrication …………….…………………………………………………… p. 2**

**SM2: Velocity profile and friction coefficient ……………………………..……… p. 4**

**SM3: Flow patterns in the meniscus ..…………………………………………………… p. 7**

**SM4: Master curve and statistics ……………………………………………………..… p. 9**

## SM1: Tip fabrication

A two-step process was developed to fabricate the non-conventional tips used in this study.

In a first step (Fig. S1), a nanofiber is milled from a conventional AFM tip (OLTESPA-R3, Bruker) using a dual beam FIB (1540 XB Cross Beam, Zeiss). The initial pyramidal tip is progressively cut by slices of 100 to 500 nm width in order to keep only the front edge of the pyramid. It results in a fiber with a rounded triangular profile. Note that, for the comparison between the experimental results and the theoretical model based on a cylindrical geometry, we use an effective theoretical radius which gives the same perimeter as the actual tip. Radius as small as 25 nm can be fabricated but, in this study, we used tips of 80 nm or 85 nm radius, which are large enough to accommodate enough defects.

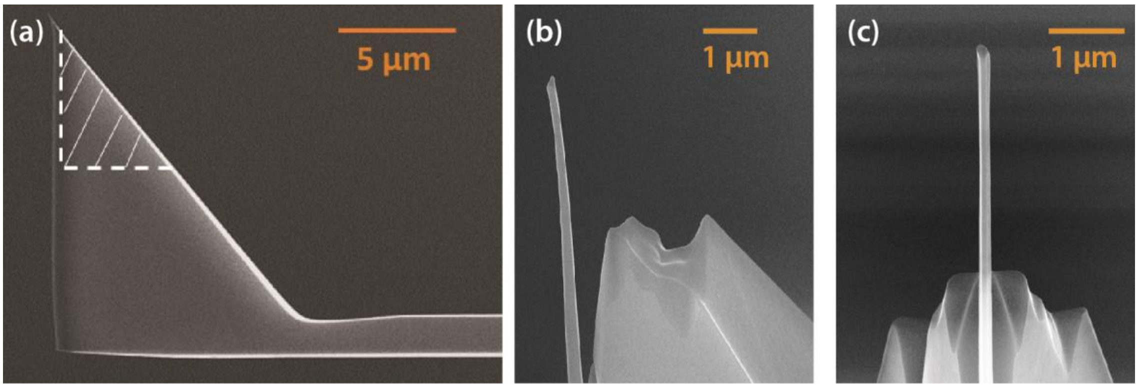


**Figure S1:** (a) Lateral SEM image of a OLTESPA-R3 (Bruker) tip. The hatched area represent the zone removed by FIB to carve the nanofiber; (b) – (c) Lateral and face view of a nanofiber after milling.

In a second step, defects are built on the nanofiber in order to pin the meniscus. This is achieved by Electron Beam Induced Deposition (EBID) using an ELPHY MultiBeam (Raith) and the gas injection system of the FIB. A platinum precursor gas injected close to the tip is decomposed by the electron beam, leaving platinum on the tip. Regular annular defects can not be achieved because a continuous motion of the electron beam results in a deposit which does not stick to the tip surface but rather forms a needle perpendicular to the tip. In order to solve

this issue, discontinuous defects are built, as shown in Figure S2. Spots with diameter ranging from 10 nm to 40 nm can be achieved. The distance between spots was adjusted in order to get the closest possible spots. Interestingly, due to the partial transparency of the thin nanofibers to electrons, thinner defects are also deposited on the back side of the tip. As a consequence of the annular defect inhomogeneity, the contact line can depin for a contact angle $\theta_{break}$ larger than the theoretical value $\theta_{crit}$. Note that the defects rings form an angle of 11° with respect to the perpendicular to the tip axis in order to compensate for the inclination of the tip in the AFM head and insuring that the defect is perpendicular to the liquid interface.

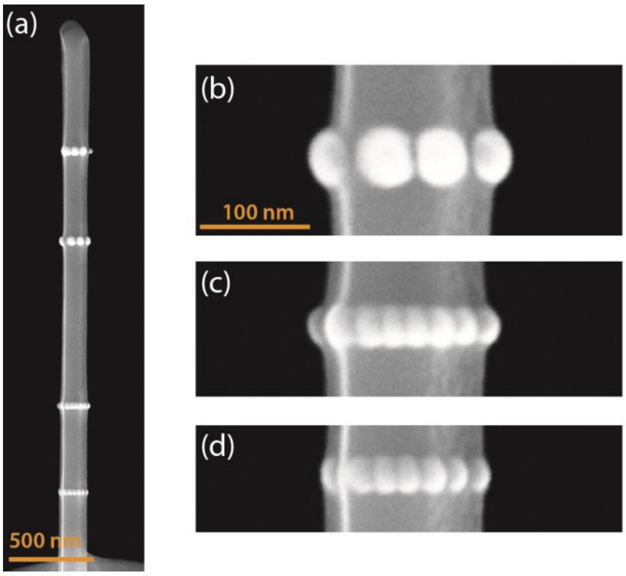


**Figure S2:** (a) SEM image of the same tip as in Fig. SM1 with 4 rings of defects deposited by EBID; (b) – (d) Zooms on the three lower defects.

## SM2: Velocity profile and friction coefficient

We consider the flow induced by the interface motion of a liquid meniscus anchored on a cylinder rod, of radius $R$, oscillating along its axis, $z$. The meniscus contact line is pinned on an annular topographical defect of radius $r_0$. In the frame of reference attached to the cylinder, the velocity field is solution, for a purely viscous Newtonian liquid under the lubrication approximation, of the Stokes equation

$$\partial_z P = \eta \Delta_r v, \tag{SI1}$$

where $P$ is the hydrodynamic pressure, $\eta$ is the fluid viscosity and $v$ is the velocity component in the $z$ direction. Equation (SI1), together with a no-slip boundary condition at the rod's surface, at $r = R$, and a no-stress boundary condition at the free interface, at $r = h(z)$, relates the velocity field to the hydrodynamic pressure gradient through the equation:

$$v(r,z) = \frac{\partial_z P(z)\left(r^2 - 2h^2(z)\ln\left(\frac{r}{R}\right) - R^2\right)}{4\,\eta}. \tag{SI2}$$

Furthermore, the velocity field is related to the interface profile through the mass conservation equation

$$\partial_t(\pi h^2) + \partial_z \int_R^{h(z)} dr\, v(r,z)\, r = 0. \tag{SI3}$$

From Eq. (SI3) we derive the pressure gradient inside the meniscus

$$\partial_z P(z) = -\frac{8\eta \int_0^z du\, \partial_t(h^2)}{R^4 + 3h^2 - 4h^2R^2 - 4h^4\ln\left(\frac{h}{R}\right)}, \tag{SI4}$$

which, in turns, gives the velocity profile as a function of the interface profile

$$v(r,z) = \frac{2\left(R^2 + 2h^2\ln\left(\frac{r}{R}\right) - r^2\right)\int_0^z du\, \partial_t(h^2)}{R^4 + 3h^2 - 4h^2R^2 - 4h^4\ln\left(\frac{h}{R}\right)}. \tag{SI5}$$

Since the capillary number is small ($Ca = A\,\omega\eta/\gamma \sim 10^{-3}$) we assume that viscous effects do not affect the shape of the liquid interface. The meniscus profile is therefore solution of the Laplace equation resulting from the balance between capillary and hydrostatic pressures, which yields the well-known catenary shape

$$h(z) = (R + r_0)\cos\theta\cosh\left(\frac{z}{(R + r_0)\cos(\theta)} - \ln\left[\frac{\cos(\theta)}{1 + \sin(\theta)}\right]\right), \tag{SI6}$$

where $\theta$ is the wetting contact angle of the meniscus.

As the contact line is pinned during the rod oscillation, the meniscus height, $Z_0(\theta)$, oscillates around its mean position, $Z_0(\bar{\theta})$, with $Z_0(\theta[t]) = Z_0(\bar{\theta}) + A\cos(\omega t)$, where $\bar{\theta}, A$ and $\omega$ are respectively the mean contact angle, the amplitude and the angular frequency of the oscillation. Together with the expression of $Z_0(\theta)$, which reads for small contact angle

$$Z_0(\theta) = (R + r_0)\cos\theta\left[\ln\left(\frac{4l_c}{R+r_0}\right) - \gamma_E\right], \tag{SI7}$$

we derive thus the temporal evolution of the contact angle

$$\cos\theta = \cos\bar{\theta} + \frac{A\cos(\omega t)}{(R + r_0)\left[\ln\left(\frac{4l_c}{R + r_0}\right) - \gamma_E\right]}. \tag{SI8}$$

Hence, Eqs. (SI5), (SI6) and (SI8) give the velocity profile inside the meniscus. Note that our model is meant to deal with positive contact angles only, even if the defect thickness could in principle allow slightly negative ones. From Eq. (SI8) we obtain therefore a critical contact angle, $\theta_{crit}$, corresponding to the minimum value of $\bar{\theta}$ allowed by the model, with

$$\cos\theta_{crit} = 1 - \frac{A}{(R + r_0)\left[\ln\left(\frac{4l_c}{R + r_0}\right) - \gamma_E\right]}. \tag{SI9}$$

We can now determinate the friction coefficient associated with the meniscus, $\beta_{men}$. For a forced harmonic oscillator that dissipates energy through viscous damping, the mean energy loss during an oscillation cycle, $P$, is related to the friction coefficient through the relation

$$P = \frac{\beta_{men}\,(A\omega)^2}{2}. \tag{SI10}$$

Furthermore, $P$ is given, for a viscous Newtonian liquid under lubrication approximation, by

$$P = \left\langle \eta \oint_V (\partial_r v)^2\, dV \right\rangle_t, \tag{SI11}$$

where $\langle\quad\rangle_t$ designates the temporal average over an oscillation cycle. Combining Eqs. (SI10) and (SI11) we obtain

$$\beta_{mean} = \left\langle \frac{2\eta}{(A\omega)^2} \oint_V (\partial_r v)^2\, dV \right\rangle_t. \tag{SI12}$$

**The case of small amplitude**

We consider the asymptotic limit of small oscillation amplitude where $\sin\theta(t) \simeq \sin\bar{\theta}$ and $h(\theta(t)) \simeq h(\bar{\theta})$. Under this approximation, the derivative of the contact angle $\dot{\theta}$ reads

$$\dot{\theta(t)} \simeq \frac{A\sin(\omega t)}{\sin\bar{\theta}(R+r_0)\left[\ln\left(\frac{4l_c}{R+r_0}\right) - \gamma_E\right]}, \tag{SI13}$$

and the normalized viscous stress is given by the equation

$$\partial_r v \simeq \frac{4\dot{\theta}(h^2/r - r)\int_0^{h(z)} du\, \partial_{\bar{\theta}}(h^2)}{R^4 + 3h^2 - 4h^2R^2 - 4h^4\ln\left(\frac{h}{R}\right)} = A\,\tilde{\sigma}_{rz}, \tag{SI14}$$

where we introduce $\tilde{\sigma}_{rz}(r,z,\bar{\theta}) = \frac{4\sin(\omega t)\left(\frac{h^2}{r}-r\right)\int_0^{h(z)} du\,\partial_{\bar{\theta}}(h^2)}{\sin\bar{\theta}(R+r_0)\left[\ln\left(\frac{4l_c}{R+r_0}\right)-\gamma_E\right]\left(R^4+3h^2-4h^2R^2-4h^4\ln\left(\frac{h}{R}\right)\right)}$. Since $\partial_r v$ is proportional to the amplitude $A$, we obtain from Eq. (SI12) that $\beta_{mean}$ does not depend on $A$ in the asymptotic case of small amplitude. However, the Taylor expansion of Eq. (SI9) shows that the critical contact angle , $\theta_{crit}$, varies as the square root of $A$ with

$$\theta_{crit} = \sqrt{\frac{2A}{(R+r_0)\left[\ln\left(\frac{4l_c}{R+r_0}\right) - \gamma_E\right]}}. \tag{SI15}$$

## SM3: Flow patterns inside the meniscus

The hydrodynamic model described in the paper provides a comprehensive description of flow patterns in an oscillating nanomeniscus which lead to the measured friction coefficient. The flow is mainly influenced by two parameters: the mean contact angle $\bar{\theta}$ and the defect size $r_0$, whose influence are discussed below.

- **Influence of the mean contact angle $\bar{\theta}$**

In Fig. S3 are reported the viscous stress field inside the meniscus as the mean contact angle $\bar{\theta}$ is reduced from $\bar{\theta} = 22°$ down to $\bar{\theta} = \theta_{crit} = 6.73°$ which is the depinning contact angle associated with the conditions used in the calculation, namely $r_0 = 40$ nm and $A = 10$ nm. The maximum stress is obtained at the fiber surface at a distance of about $2.5\, r_0$ from the contact line. The decrease of contact angle significantly increases the value of the stress without any noticeable modification of the position of its localization inside the nanomeniscus.

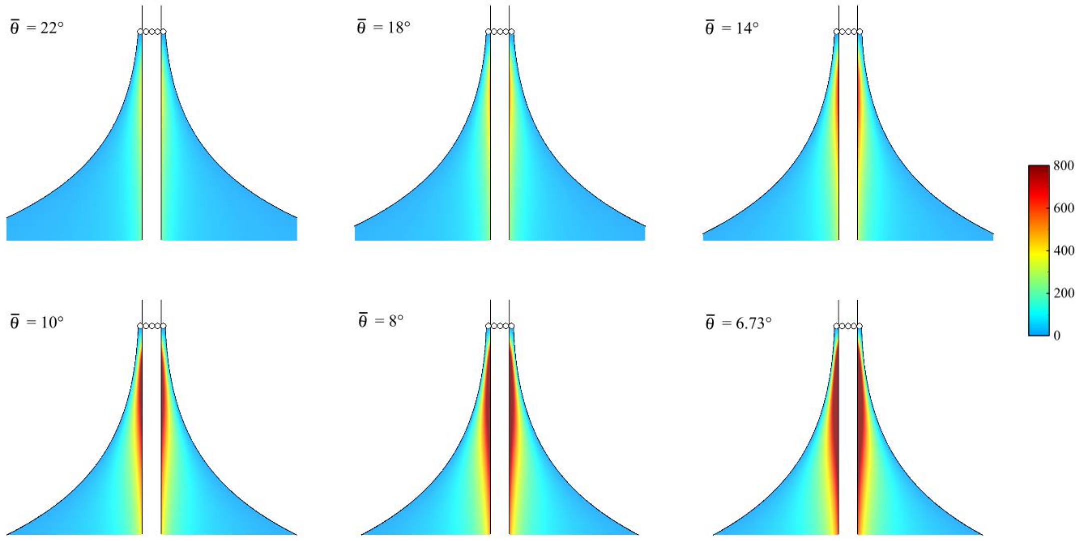


**Figure S3:** Viscous stress field $\eta\partial_r v$ (color gradient), computed at t = 0, for 6 different contact angles and $R = 100\, nm$, $r_0 = 30\, nm$, $l_c = 2\, mm$, $A = 10\, nm$, $f = 65\, kHz$ and $\eta = 30\, mPa.s$. Color bar in Pa.

- **Influence of the defect size**

The defect height $r_0$ has a strong influence on the dissipation pattern as shown in Fig. S4. A decrease of defect size leads to a strong enhancement of the viscous stress inside the meniscus, which can be understood by the fact that small defects results in smaller films thickness at the contact line and consequently larger velocity gradients. Another striking effect is that the defect size also affects the localization of the viscous field which becomes concentrated closer from the contact line as $r_0$ is decreased. This effects is not straightforward and may have important consequences on the wetting on surfaces with defects.

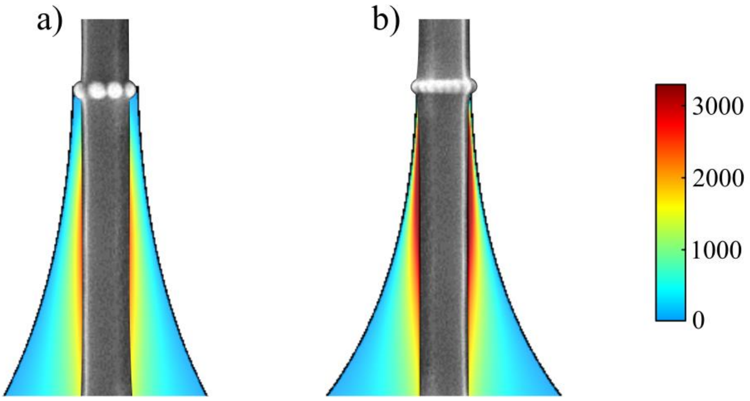


**Figure S4:** Viscous stress field $\eta \partial_r v$ (color gradient), computed at the critical contact angle value and t = 0s , for 2 different defect sizes : (a) $r_0 = 40\ nm$ and (b) $r_0 = 10\ nm$. The parameters used are $R = 100\ nm$, $l_c = 2\ mm$, $A = 10\ nm$, $f = 65\ kHz$ and $\eta = 30\ mPa.s$. Color bar in Pa.

## SM4: Master curve and statistics

As shown in the paper, the experimental conditions, namely the defect size $r_0$ and the oscillation amplitude $A$, have a small influence on the friction coefficient. We therefore reported in Fig. SM5 around twenty curves performed using different tips, defects, liquids and amplitude. All curves superpose in a rather thin zone which is nicely bounded by the theoretical curves giving the extreme cases within the range of experimental conditions (10 nm $\leq r_0 \leq$ 50 nm and 6 nm $\leq A \leq$ 33 nm). The higher dissipation is obtained for small defect and high amplitude ($r_0 = 5$ nm and $A = 33$ nm).

From all the measurements (more than ninety), we extracted a histogram of the values of $\beta_{bottom}$ used in the fits (inset Fig. S5). The mean value of $\beta_{bottom} = (7 \pm 3.5)\eta R$ is consistent with the theoretical expression, $\beta_{bottom} = 8\eta R$, expected for a flat tip end. However, the ill-defined tip end geometry leads to a strong dispersion of the experimental results which hinders a more quantitative comparison with the theory.

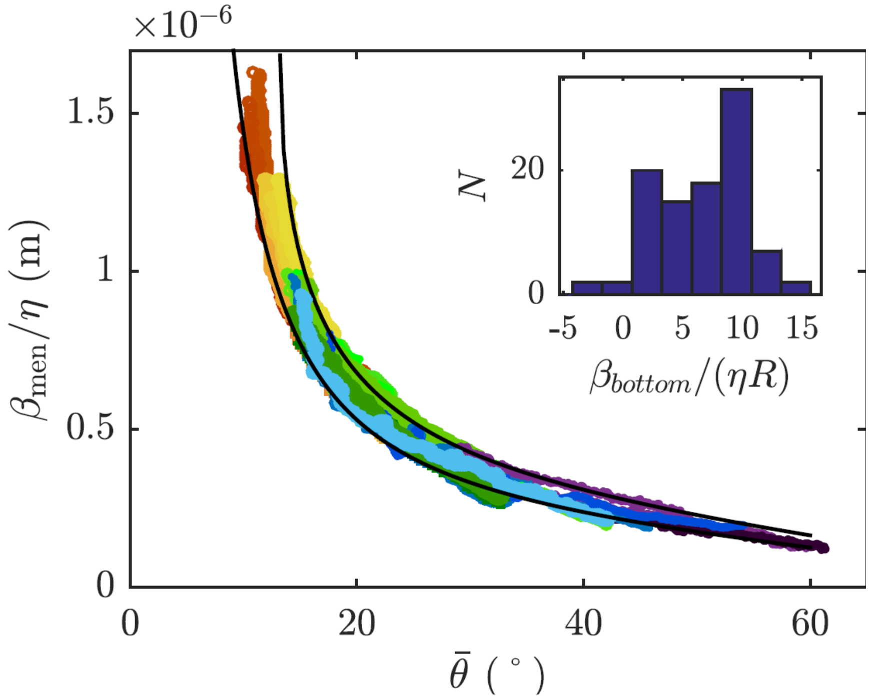


**Figure S5:** (a) Superposition of all the experimental curves. In order to visualize different curves, the color is related to the $\theta_{break}$ value. The range of theoretical values appears in

grey and is limited by two solid lines ($r_0 = 5\ nm$, $A = 33\ nm$ for the higher one and $r_0 = 50\ nm$, $A = 6\ nm$ for the lower one); (b) Histogram of the $\beta_{bottom}/\eta R$ values extracted from the experimental data.
